# Supplementary material for: Estimating dimension of inertial manifold from unstable periodic orbits
Source: arXiv:1604.01859 ancillary file (2016-04-07)
Supplement: Supplementary file 1 [file upodim-suppl.pdf]

# Supplementary Material for "Estimating dimension of inertial manifold from unstable periodic orbits"

X. Ding,[1] H. Chaté,[2,3] P. Cvitanović,[1] E. Siminos,[4,5] and K. A. Takeuchi[6,*]

[1] *Center for Nonlinear Science, School of Physics, Georgia Institute of Technology, Atlanta, GA 30332-0430, USA*
[2] *Service de Physique de l'Etat Condensé, CEA, CNRS, Université Paris-Saclay, CEA-Saclay, 91191 Gif-sur-Yvette, France*
[3] *Beijing Computational Science Research Center, Beijing 100094, China*
[4] *Max-Planck Institute for the Physics of Complex Systems, Nöthnitzer Str. 38, D-01187 Dresden, Germany*
[5] *Department of Physics, Chalmers University of Technology, Gothenburg, Sweden*
[6] *Department of Physics, Tokyo Institute of Technology, 2-12-1 Ookayama, Meguro-ku, Tokyo 152-8551, Japan*

(Dated: April 6, 2016)

## I. IN-SLICE FLOQUET VECTORS

This section describes how the in-slice Floquet vectors $|\hat{\boldsymbol{e}}_j(\hat{\mathbf{x}})\rangle$ are defined and obtained from the original Floquet vectors $|\boldsymbol{e}_j(\mathbf{x})\rangle$ (bra-ket notation is used). As in the Letter, we consider an autonomous flow $|\mathbf{x}(t)\rangle = f^t\,|\mathbf{x}(0)\rangle$ in $d$-dimensional phase space. The Kuramoto-Sivashinsky equation formally corresponds to $d=\infty$, but in practice numerical integration is performed in a finite-dimensional phase space, whose dimensionality $d$ is set by the cutoff wavenumber chosen in the pseudospectral method. In any case, $|\mathbf{x}(t)\rangle$ represents the field $u(x,t)$, which is also described by its Fourier components

$$a_k(t) \equiv \frac{1}{L}\int_0^L u(x,t)e^{-iq_k x}, \tag{S1}$$

with $q_k = 2\pi k/L$ and $a_0(t)=0$. Within this formalism, a periodic orbit $|\mathbf{x}(0)\rangle$ is a fixed point of the map $f^{T_p}$, with $T_p$ the period of the orbit. Its Floquet multipliers $\Lambda_j$ and Floquet vectors $|\boldsymbol{e}_j(\mathbf{x})\rangle$ are the eigenvalues and eigenvectors, respectively, of the corresponding Jacobian $J^{T_p}$. Pre-periodic orbits and relative periodic orbits can also be dealt with straightforwardly, by replacing $f^{T_p}$ with $Rf^{T_p}$ and $g(\theta_p)f^{T_p}$, respectively, with reflection $\sigma$ and spatial translation $g(\theta_p)$ as defined in the Letter. Therefore, in the following, we describe the case of periodic orbits for the sake of simplicity.

Here we focus on the invariance under spatial translation $u(x,t)\to u(x+\ell,t)$, which amounts to a rotation $a_k(t)\to e^{iq_k\ell}a_k(t)$ in Fourier space, described by the operator $g(2\pi\ell/L)$. To reduce the marginal dimension due to this symmetry, we send all trajectories and orbits to the $(d-1)$-dimensional hyperplane

$$\mathrm{Im}(a_1(t)) = 0, \quad \mathrm{Re}(a_1(t)) > 0, \tag{S2}$$

which is called the first Fourier-mode slice [S1]. This is realized by transformation

$$|\hat{\mathbf{x}}(t)\rangle \equiv g(-\theta(\mathbf{x}(t)))\,|\mathbf{x}(t)\rangle \tag{S3}$$

with $\theta(\mathbf{x}(t)) = \arg a_1(t)$.

First we consider infinitesimal perturbations to $|\mathbf{x}(t)\rangle$, denoted here by $|\delta\mathbf{x}(t)\rangle$. Using Eq. (S3), one can show that $|\delta\mathbf{x}(t)\rangle$ is transformed to

$$|\delta\hat{\mathbf{x}}(t)\rangle' \equiv h(\mathbf{x}(t))g(-\theta(\mathbf{x}(t)))\,|\delta\mathbf{x}(t)\rangle\,, \tag{S4}$$

with

$$h(\mathbf{x}) \equiv 1 - \frac{|T\mathbf{x}\rangle\,\langle T\mathbf{x}_0|}{\langle T\mathbf{x}_0|T\mathbf{x}\rangle}. \tag{S5}$$

Here, $T$ is the generator defined by $g(\theta)\equiv e^{T\theta}$, the inner product is

$$\langle\mathbf{x}|\mathbf{x}'\rangle \equiv \frac{1}{L}\int_0^L u^*(x)u'(x)dx = \sum_k a_k^* a_k', \tag{S6}$$

and $\mathbf{x}_0$ is a reference point on the slice [S1], which therefore satisfies $\langle\delta\hat{\mathbf{x}}(t)|T\mathbf{x}_0\rangle = 0$. Since we use the first Fourier-mode slice (S2), we can take $\mathbf{x}_0 = (1,0,\cdots,0)$ in the Fourier representation. Note that, since the dimensionality of the slice is one less than that of the phase space, so is the dimensionality of the in-slice perturbations. This is reflected by the fact that $\langle T\mathbf{x}_0|\,h(\mathbf{x}) = 0$, or $\sum_i t_i' h_i(\mathbf{x}) = 0$, where $h_i(\mathbf{x})$ is the $i$th row vector of $h(\mathbf{x})$ and $t_i'$ the $i$th component of $\langle T\mathbf{x}_0|$. Therefore, by rank factorization, one obtains

* kat@kaztake.org

$$h(\mathbf{x}) = \begin{bmatrix} h_1 \\ \vdots \\ h_{i_0-1} \\ h_{i_0} \\ h_{i_0+1} \\ \vdots \\ h_d \end{bmatrix} = \begin{bmatrix} 1 & & & & & & \\ & \ddots & & & & O & \\ & & 1 & & & & \\ -\frac{t'_1}{t'_{i_0}} & \cdots & -\frac{t'_{i_0-1}}{t'_{i_0}} & -\frac{t'_{i_0+1}}{t'_{i_0}} & \cdots & -\frac{t'_d}{t'_{i_0}} \\ & & & 1 & & \\ & O & & & \ddots & \\ & & & & & 1 \end{bmatrix} \begin{bmatrix} h_1 \\ \vdots \\ h_{i_0-1} \\ h_{i_0+1} \\ \vdots \\ h_d \end{bmatrix} \equiv P\hat{h}(\mathbf{x}), \tag{S7}$$

with $d \times (d-1)$ matrix $P$, $(d-1) \times d$ matrix $\hat{h}(\mathbf{x})$, and $i_0$ chosen such that $t'_{i_0} \neq 0$. For the first Fourier-mode slice adopted here, all the components of $\langle T\mathbf{x}_0|$ except $t'_2$ are zero [S1], so that $i_0 = 2$.

Now let us define the $(d-1)$-dimensional in-slice perturbation $|\delta\hat{\mathbf{x}}(t)\rangle$ by

$$|\delta\hat{\mathbf{x}}(t)\rangle \equiv \hat{h}(\mathbf{x}(t))g(-\theta(\mathbf{x}(t)))\,|\delta\mathbf{x}(t)\rangle\,. \tag{S8}$$

By construction, there is one-to-one correspondence between $|\delta\hat{\mathbf{x}}(t)\rangle'$ and $|\delta\hat{\mathbf{x}}(t)\rangle$ through the operator $P$ [see Eqs. (S4), (S7), (S8)], unless $|\delta\hat{\mathbf{x}}(t)\rangle'$ is tangent to the spatial translation, $|\delta\hat{\mathbf{x}}(t)\rangle' \propto |T\mathbf{x}\rangle$, which results in $|\delta\hat{\mathbf{x}}(t)\rangle = 0$ [see Eq. (S5)]. Therefore, $|\delta\hat{\mathbf{x}}(t)\rangle$ indeed describes the perturbation within the slice. Moreover, if we define the evolution operator $\hat{J}^t(\mathbf{x})$ by

$$|\delta\hat{\mathbf{x}}(t)\rangle = \hat{J}^t(\mathbf{x}(0))\,|\delta\hat{\mathbf{x}}(0)\rangle\,, \tag{S9}$$

similarly to

$$|\delta\mathbf{x}(t)\rangle = J^t(\mathbf{x}(0))\,|\delta\mathbf{x}(0)\rangle\,, \tag{S10}$$

with $J^t(\mathbf{x})$ being the Jacobian of $f^t(\mathbf{x})$, we obtain

$$\begin{aligned} |\delta\hat{\mathbf{x}}(t)\rangle &= \hat{h}(\mathbf{x}(t))g(-\theta(\mathbf{x}(t)))J^t(\mathbf{x}(0))\,|\delta\mathbf{x}(0)\rangle \\ &= \hat{J}^t(\mathbf{x}(0))\hat{h}(\mathbf{x}(0))g(-\theta(\mathbf{x}(0)))\,|\delta\mathbf{x}(0)\rangle\,. \end{aligned} \tag{S11}$$

For a periodic orbit of period $T_p$ (hence $\mathbf{x}(T_p) = \mathbf{x}(0)$), we have $J^{T_p}(0)\,|\boldsymbol{e}_j(\mathbf{x}(0))\rangle = \Lambda_j\,|\boldsymbol{e}_j(\mathbf{x}(0))\rangle$ with its Floquet multipliers $\Lambda_j$ and vectors $|\boldsymbol{e}_j(\mathbf{x})\rangle$. Therefore, defining

$$|\hat{\boldsymbol{e}}_j(\mathbf{x})\rangle \equiv \hat{h}(\mathbf{x})g(-\theta(\mathbf{x}))\,|\boldsymbol{e}_j(\mathbf{x})\rangle\,, \tag{S12}$$

we find that they are indeed eigenvectors of $\hat{J}^t(\mathbf{x})$, associated with the eigenvalues $\Lambda_j$ unchanged by the transformation. This justifies calling $|\hat{\boldsymbol{e}}_j(\mathbf{x})\rangle$ the in-slice Floquet vectors, associated with the Floquet multipliers $\Lambda_j$ or exponents $\lambda_j$ of the orbit. Similarly to $|\delta\hat{\mathbf{x}}(t)\rangle$, all information of the $j$th Floquet mode is retained in the corresponding in-slice Floquet mode, except that the marginal mode due to the spatial translation is excluded in the in-slice descriptions. Therefore, the number of the marginal modes, as well as the number of the entangled Floquet modes, are one less than those in the full-space descriptions.

[S1] N. B. Budanur, P. Cvitanović, R. L. Davidchack, and E. Siminos, Phys. Rev. Lett. **114**, 084102 (2015).
